# Supplementary material for: The Bolza curve and some orbifold ball quotient surfaces
Source: arXiv:1904.00793 ancillary file (2020-02-14)
Supplement: Supplementary file 1 [file Magma_KRR.pdf]

```
// This is the Magma code for the paper
// 'The Bolza curve and some orbifold ball quotient surfaces',
// by V. Koziars, X. Roulleau and C. Rito.
```

```
// Section 5.3:
```

```
R<u,v,m,n,a,b,c,d,e>:=PolynomialRing(Rationals(),9);
P<x,z>:=PolynomialRing(R,2);
f:=(u*x+v*z)^3*(m*x+n*z);
s:=Coefficients(f);
I:=ideal<R|a-s[5],b-s[4],c-s[3],d-s[2],e-s[1]>;
EliminationIdeal(I,4);
```

```
K:=Rationals();
R<a,q1,q2,m,d1,d2,n>:=PolynomialRing(K,7);
P<x,y,z>:=ProjectiveSpace(R,2);
```

```
F:=(x^2 + x*y + y^2 - x*z - y*z)^2 + a*x*y*(x + y - z)^2;
```

```
p6:=[q1,m*q1,1];
p7:=[q2,m*q2,1];
```

```
P1:=Evaluate(F,[q1,m*q1,1]);
P2:=Evaluate(F,[q2,m*q2,1]);
```

```
L1:=-y+d1*x+(m*q1-d1*q1)*z;
L2:=-y+d2*x+(m*q2-d2*q2)*z;
```

```
M1:=Matrix([JacobianSequence(F),JacobianSequence(L1)]);
M1:=Evaluate(M1,[q1,m*q1,1]);
M2:=Matrix([JacobianSequence(F),JacobianSequence(L2)]);
M2:=Evaluate(M2,[q2,m*q2,1]);
```

```
D1:=Minors(M1,2)[1];
D2:=Minors(M2,2)[1];
```

```
R1:=Evaluate(F,y,d1*x+(m*q1-d1*q1)*z);
R2:=Evaluate(F,y,d2*x+(m*q2-d2*q2)*z);
```

```
c:=Coefficients(R1);
P3:=c[1]*c[5]-1/4*c[2]*c[4]+1/12*c[3]^2;
P4:=c[1]*c[4]^2+c[2]^2*c[5]-c[2]*c[3]*c[4]+8/27*c[3]^3;
c:=Coefficients(R2);
P5:=c[1]*c[5]-1/4*c[2]*c[4]+1/12*c[3]^2;
P6:=c[1]*c[4]^2+c[2]^2*c[5]-c[2]*c[3]*c[4]+8/27*c[3]^3;
```

```
D3:=Evaluate(L1,[0,1,1]);
D4:=Evaluate(L1,[1,0,1]);
D5:=Evaluate(L2,[0,1,1]);
D6:=Evaluate(L2,[1,0,1]);
```

```

D7:=(m-d1)*(m-d2);

D8:=a*q1*q2*(q1-q2);

A:=AffineSpace(R);
S:=Scheme(A,[P1,P2,P3,P4,P5,P6,1+n*D1*D2*D3*D4*D5*D6*D7*D8]);

PrimeComponents(S);

// Section 6.1:

K:=Rationals();
R<r>:=PolynomialRing(K);
K<r>:=ext<K|r^2+2>;
P2<x,y,z>:=ProjectiveSpace(K,2);
Q:=Curve(P2,(x^2+x*y+y^2-x*z-y*z)^2-8*x*y*(x+y-z)^2);
p6:=P2![2*r,-2*r,1];
p7:=P2![-2*r,2*r,1];

L:=LinearSystem(LinearSystem(P2,2),[p6,p7]);
P3<a,b,c,d>:=ProjectiveSpace(K,3);
rho:=map<P2->P3|Sections(L)>;

Q2:=rho(P2);Q2;
C:=rho(Q);C;

sigma:=map<P3->P3|[d,b,c,a]>;
C:=rho(Q);C;
sigma(Q2) eq Q2;
sigma(C) eq C;

psi:=map<P3->P2|[a+d,b,c]>;
Cu:=psi(C);
Co:=psi(Scheme(rho(P2),[a-d]));
Co:=Curve(P2,DefiningEquations(Co));

pts:=SingularPoints(Cu);
ResolutionGraph(Cu,pts[1]);

Degree(ReducedSubscheme(Co meet Cu)) eq 3;
pt:=Points(Co meet Cu)[1];
IntersectionNumber(Co,Cu,pt) eq 4;

```
